# Supplementary material for: Are Metrics Enough? Guidelines for Communicating and Visualizing Predictive Models to Subject Matter Experts
Source: arXiv:2205.05749 source file (2025-03-17)
Supplement: Supplementary file 1 [file sec-appendix.tex]

% \section{Figures}

\begin{figure*}[!t]
    \centering
    \begin{tabular}{cc}
    	\toprule

        \textbf{KNN (Baseline)} & \textbf{XGB (In-development)} \\
        
        \midrule
        
    	%%% 1D distribution of predictions
    	% KNN
    	\includegraphics[width=.4\linewidth]{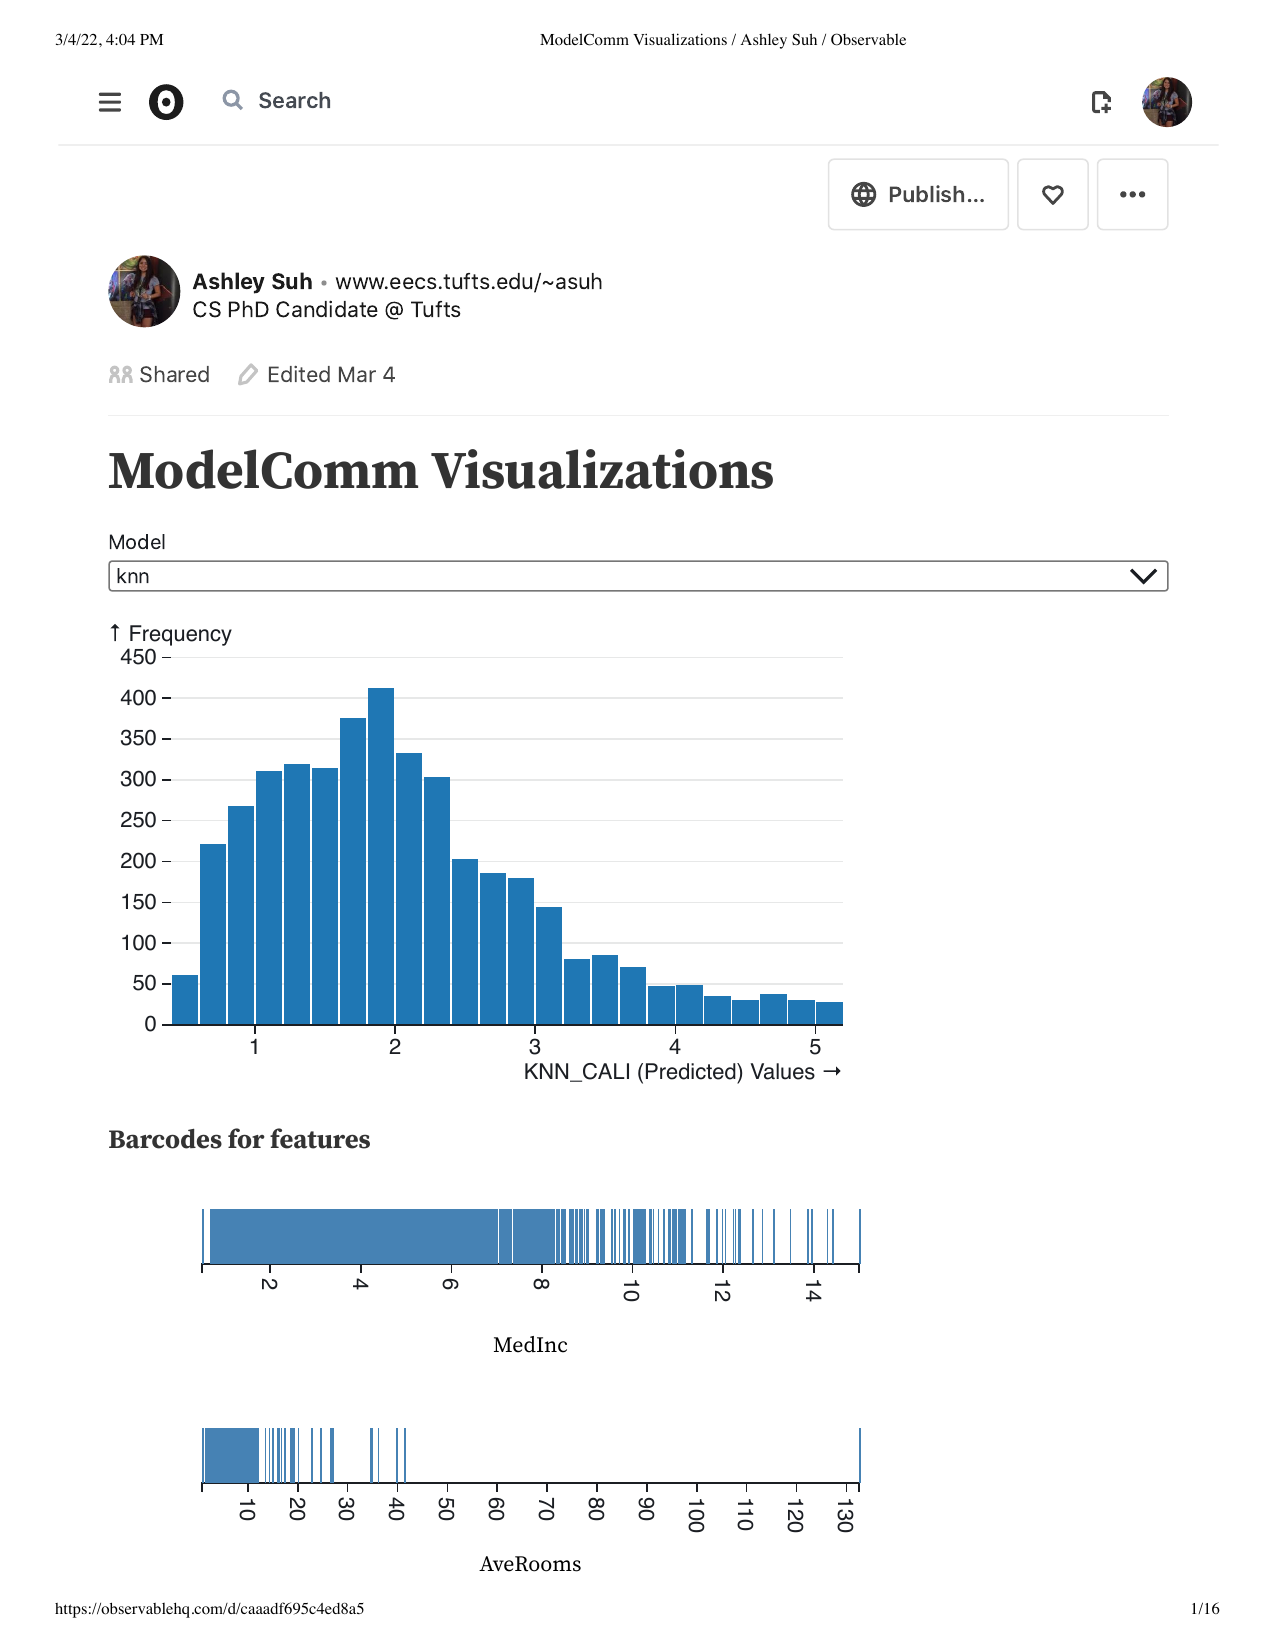}
    	% XGB
    	& \includegraphics[width=.4\linewidth]{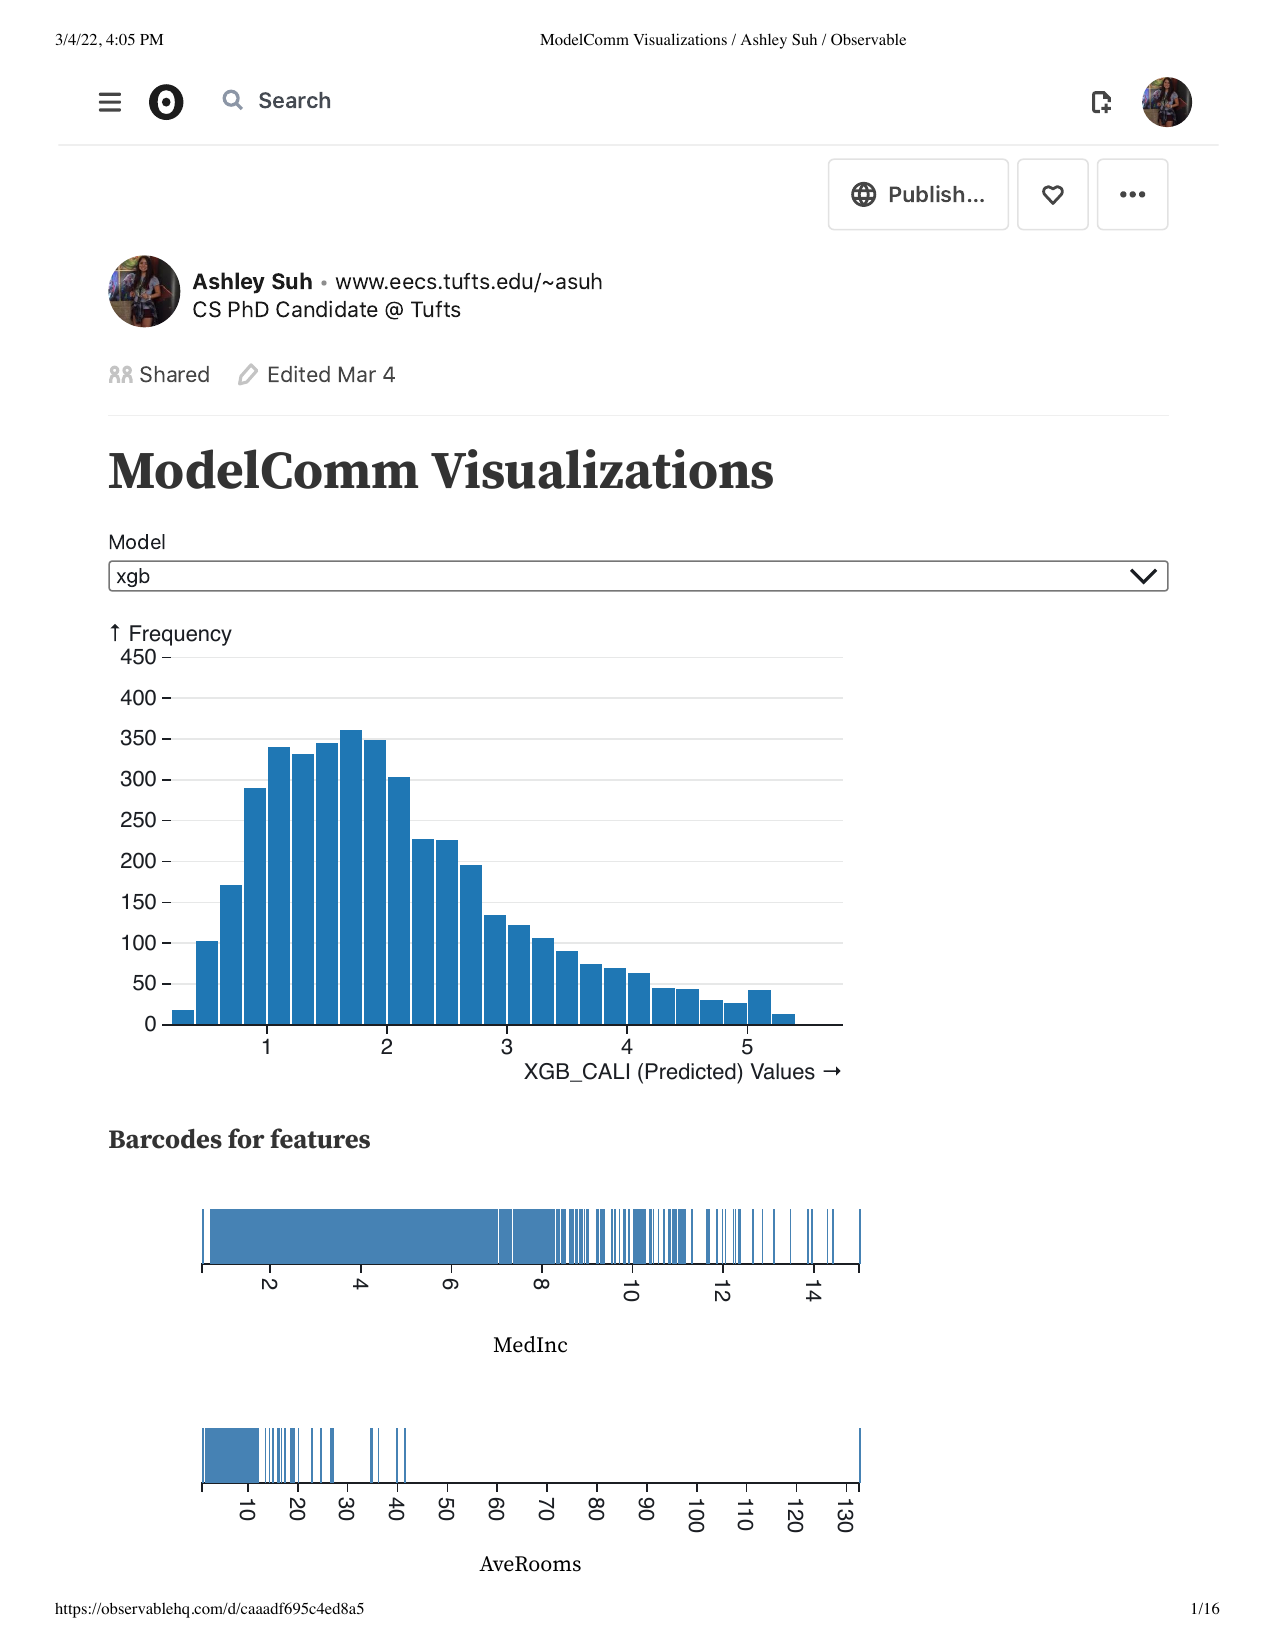} \\ 
    	
        %%% Corr scatterplot
    	% KNN
    	\includegraphics[width=.4\linewidth]{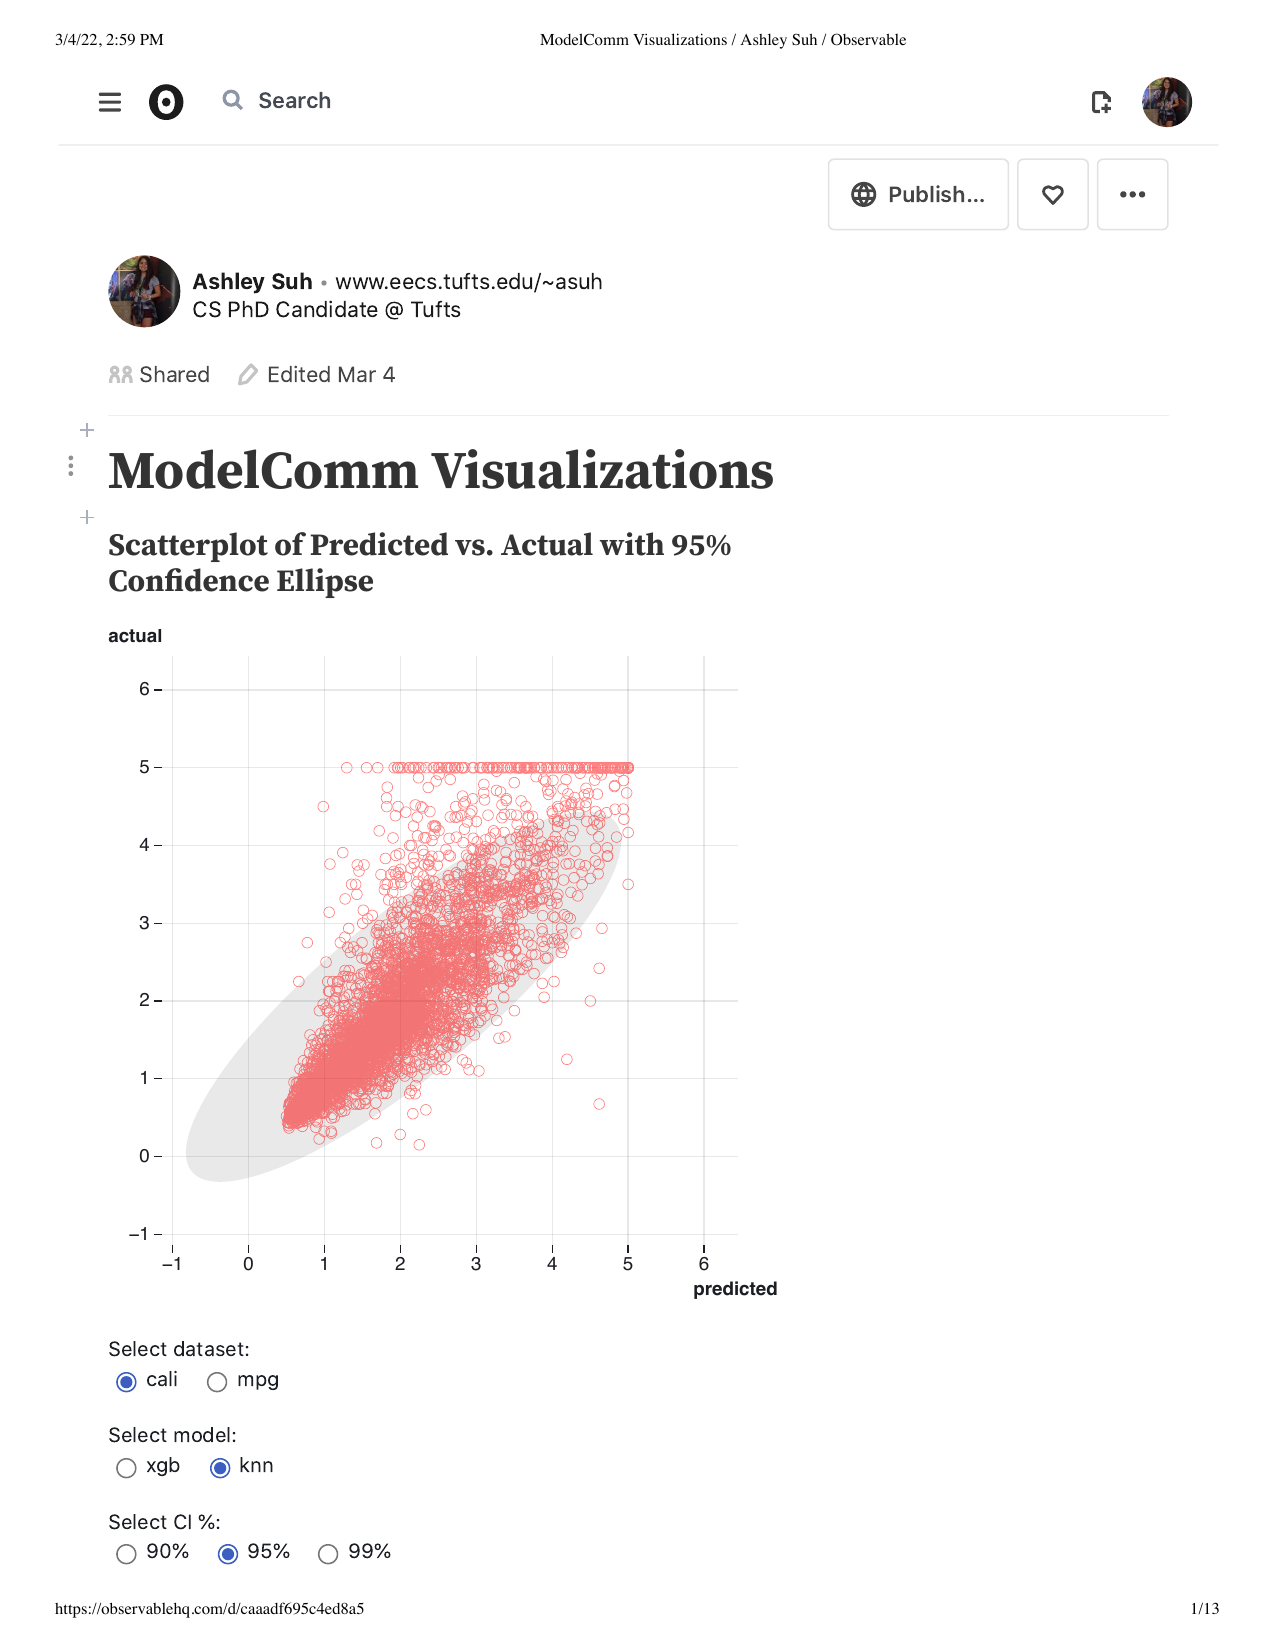}
    	% XGB
    	& \includegraphics[width=.\linewidth]{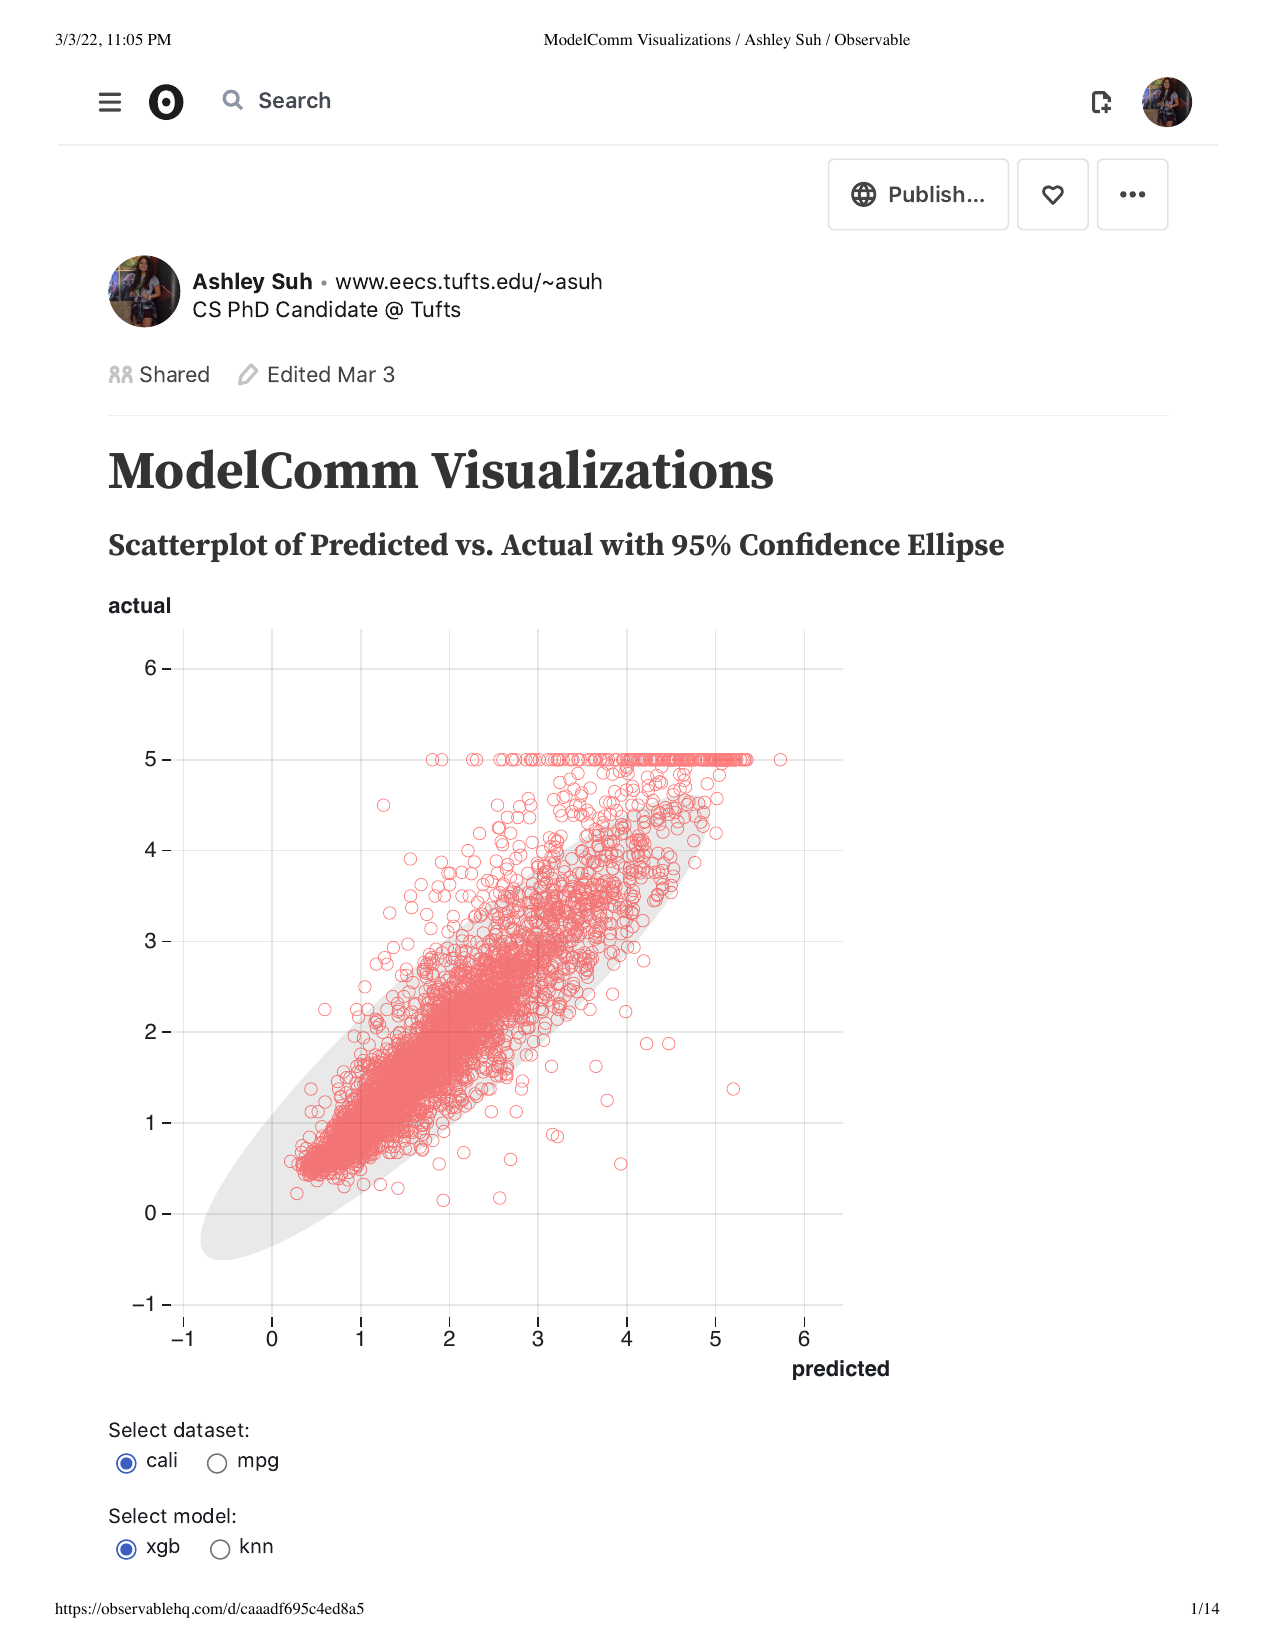} \\ 
    	
    	%%% Global error bar chart
    	% KNN
    	\includegraphics[width=.4\linewidth]{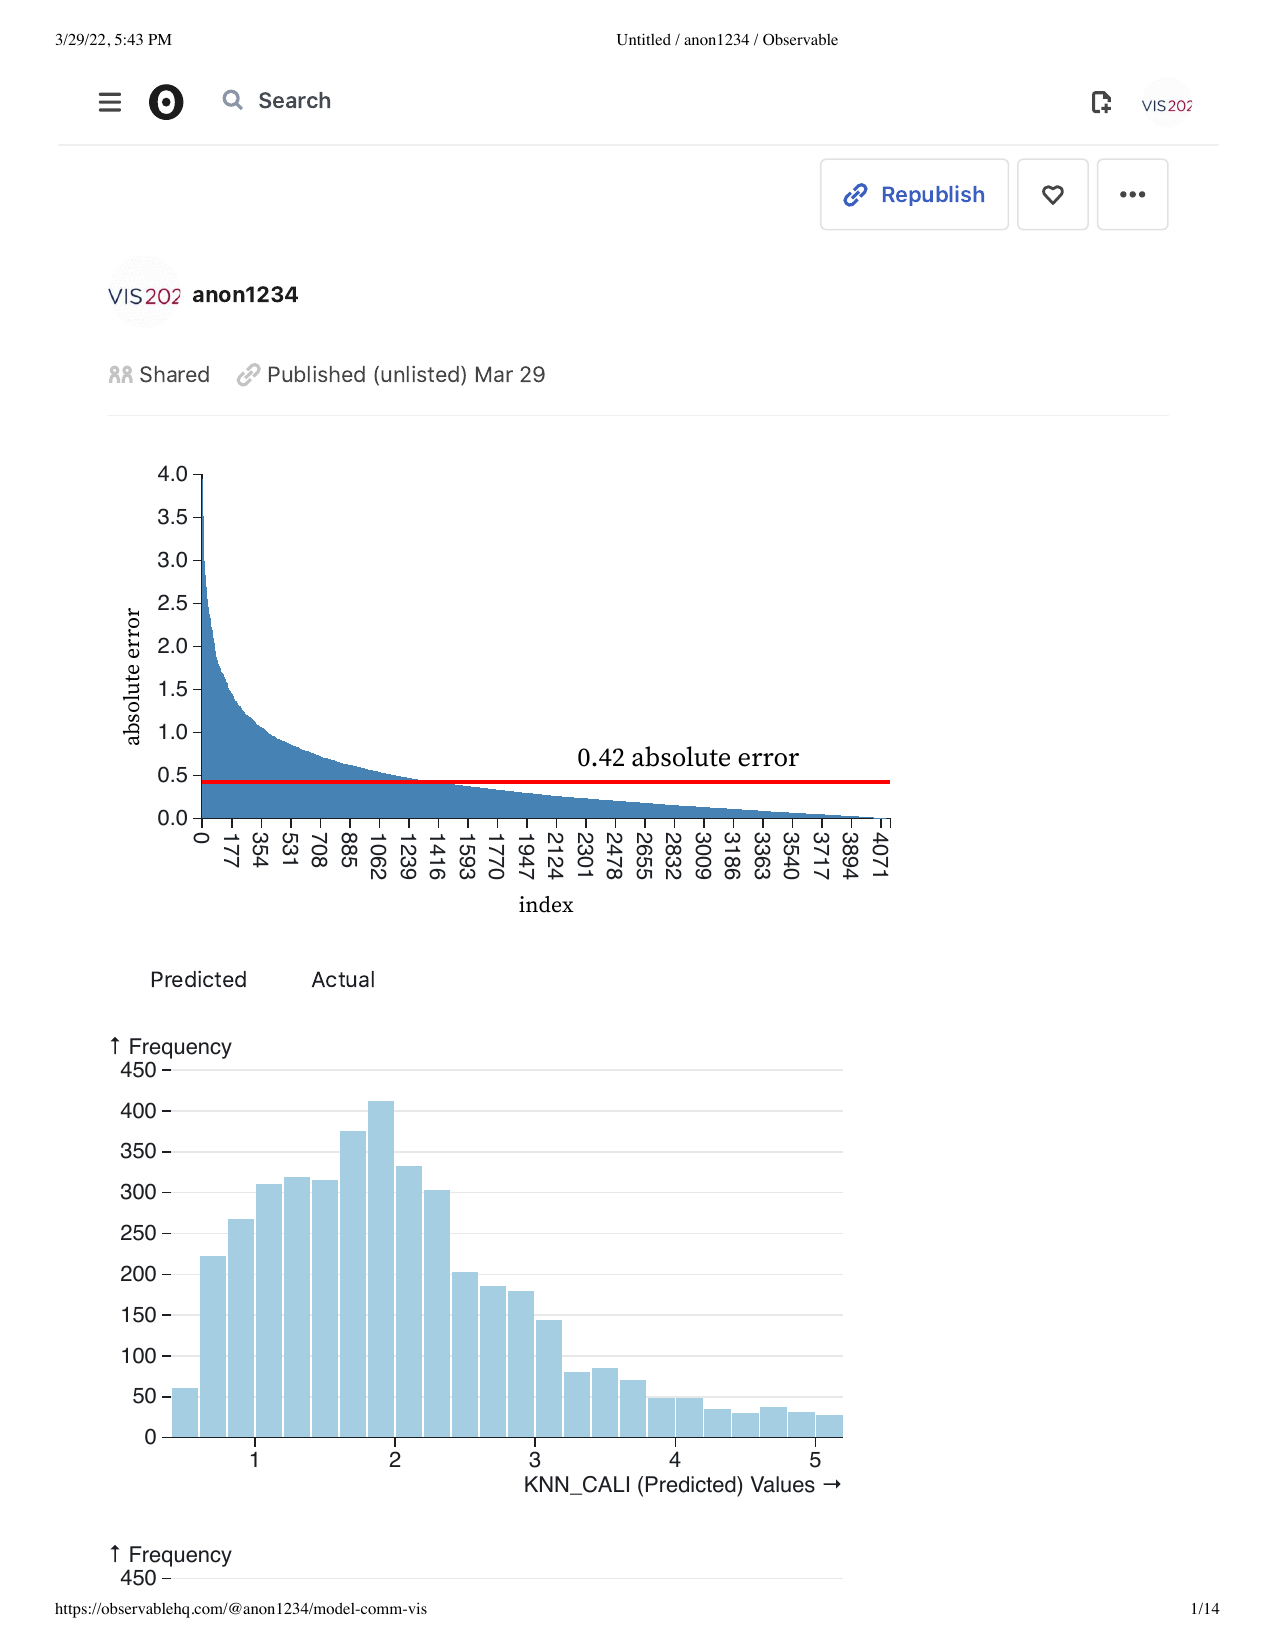}
    	% XGB
    	& \includegraphics[width=.4\linewidth]{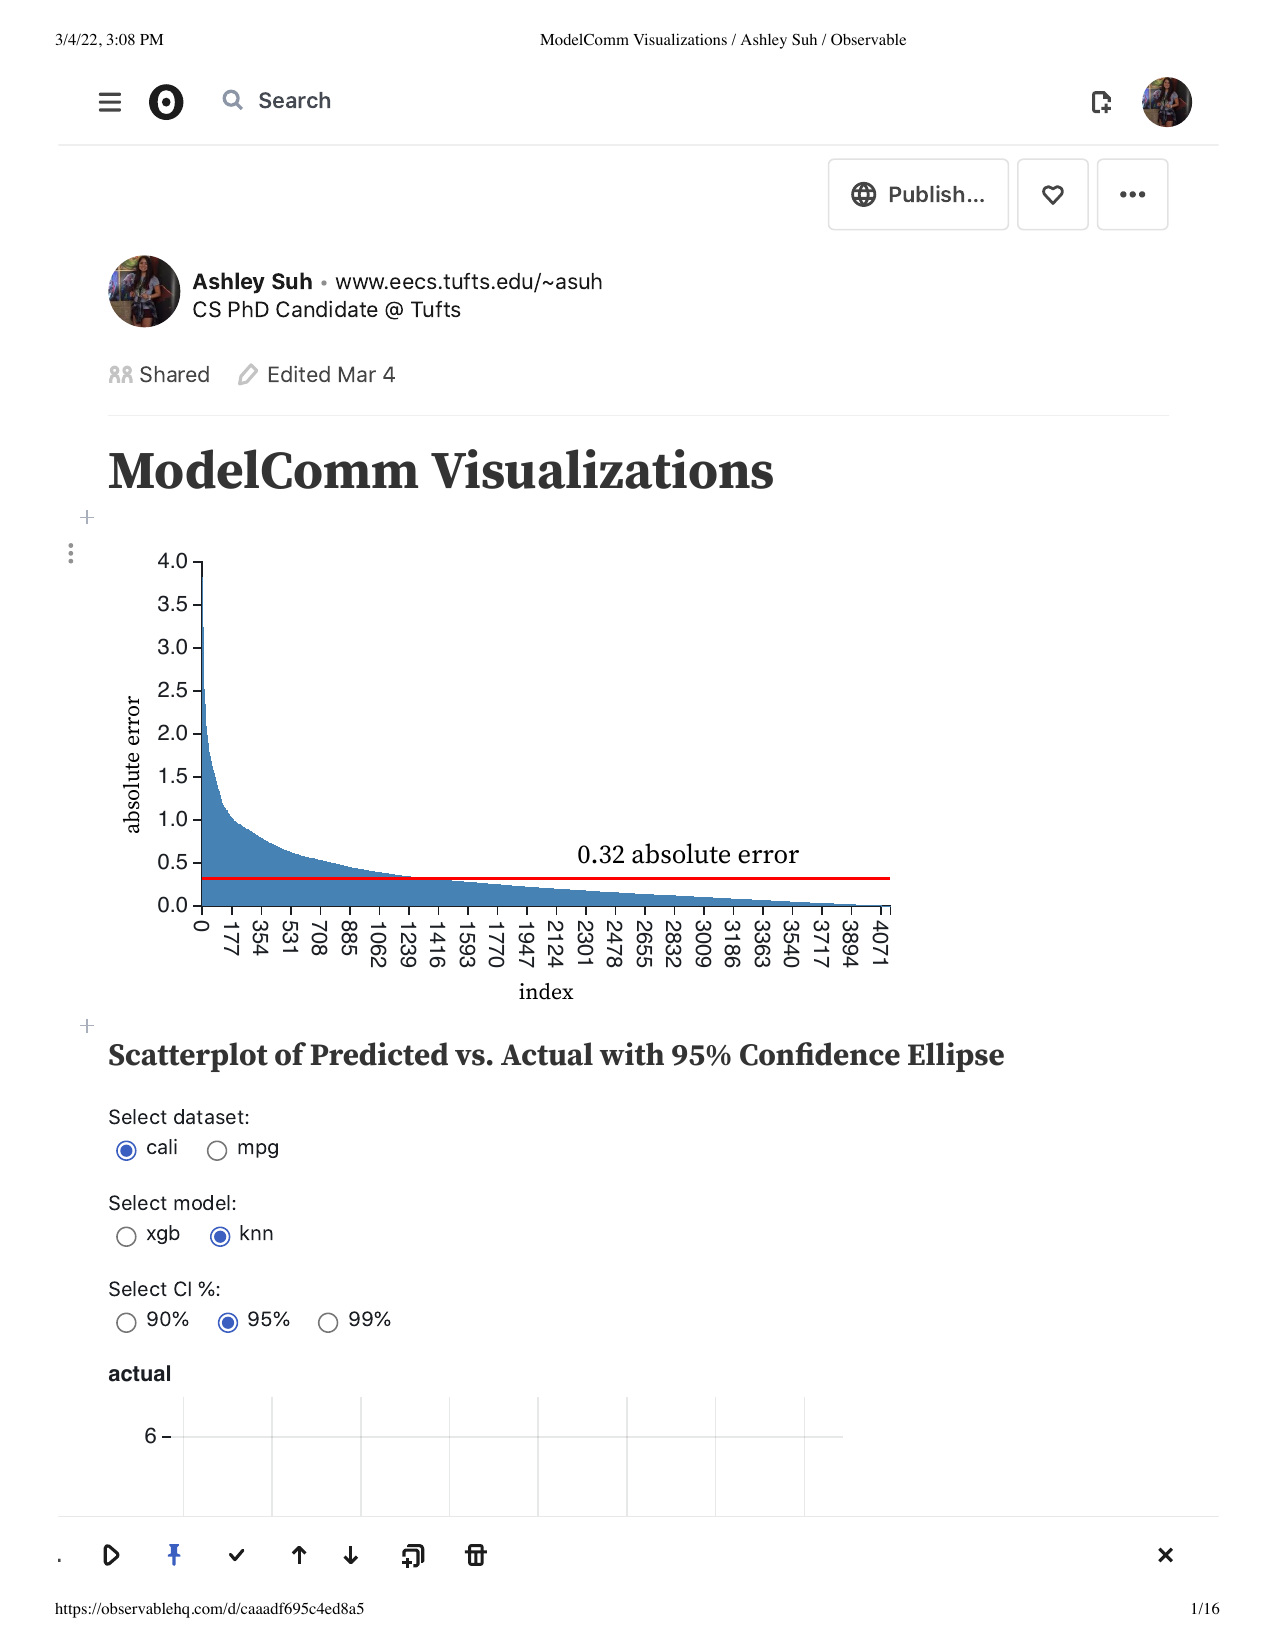} \\ 
    	
    	%%% Dual KDE plots
    	% KNN
    	\includegraphics[width=.4\linewidth]{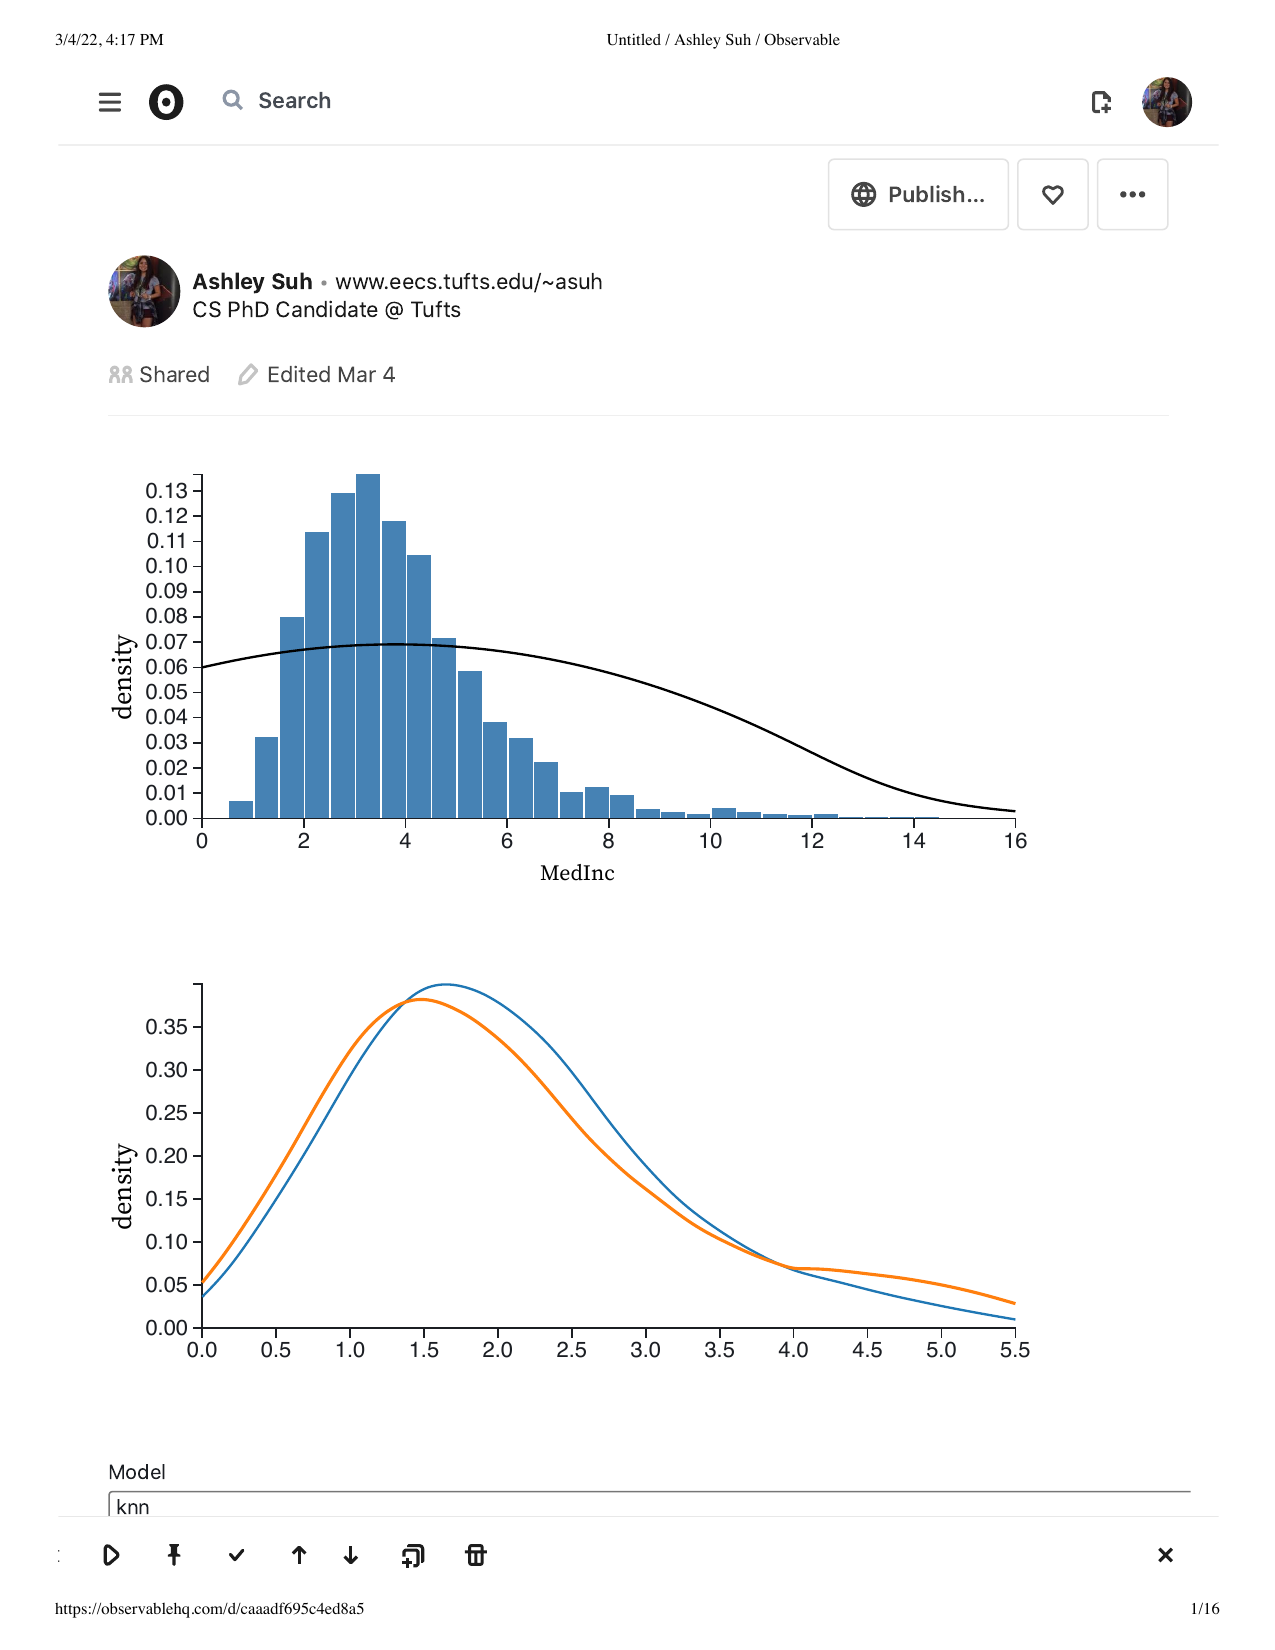}
    	% XGB
    	& \includegraphics[width=.4\linewidth]{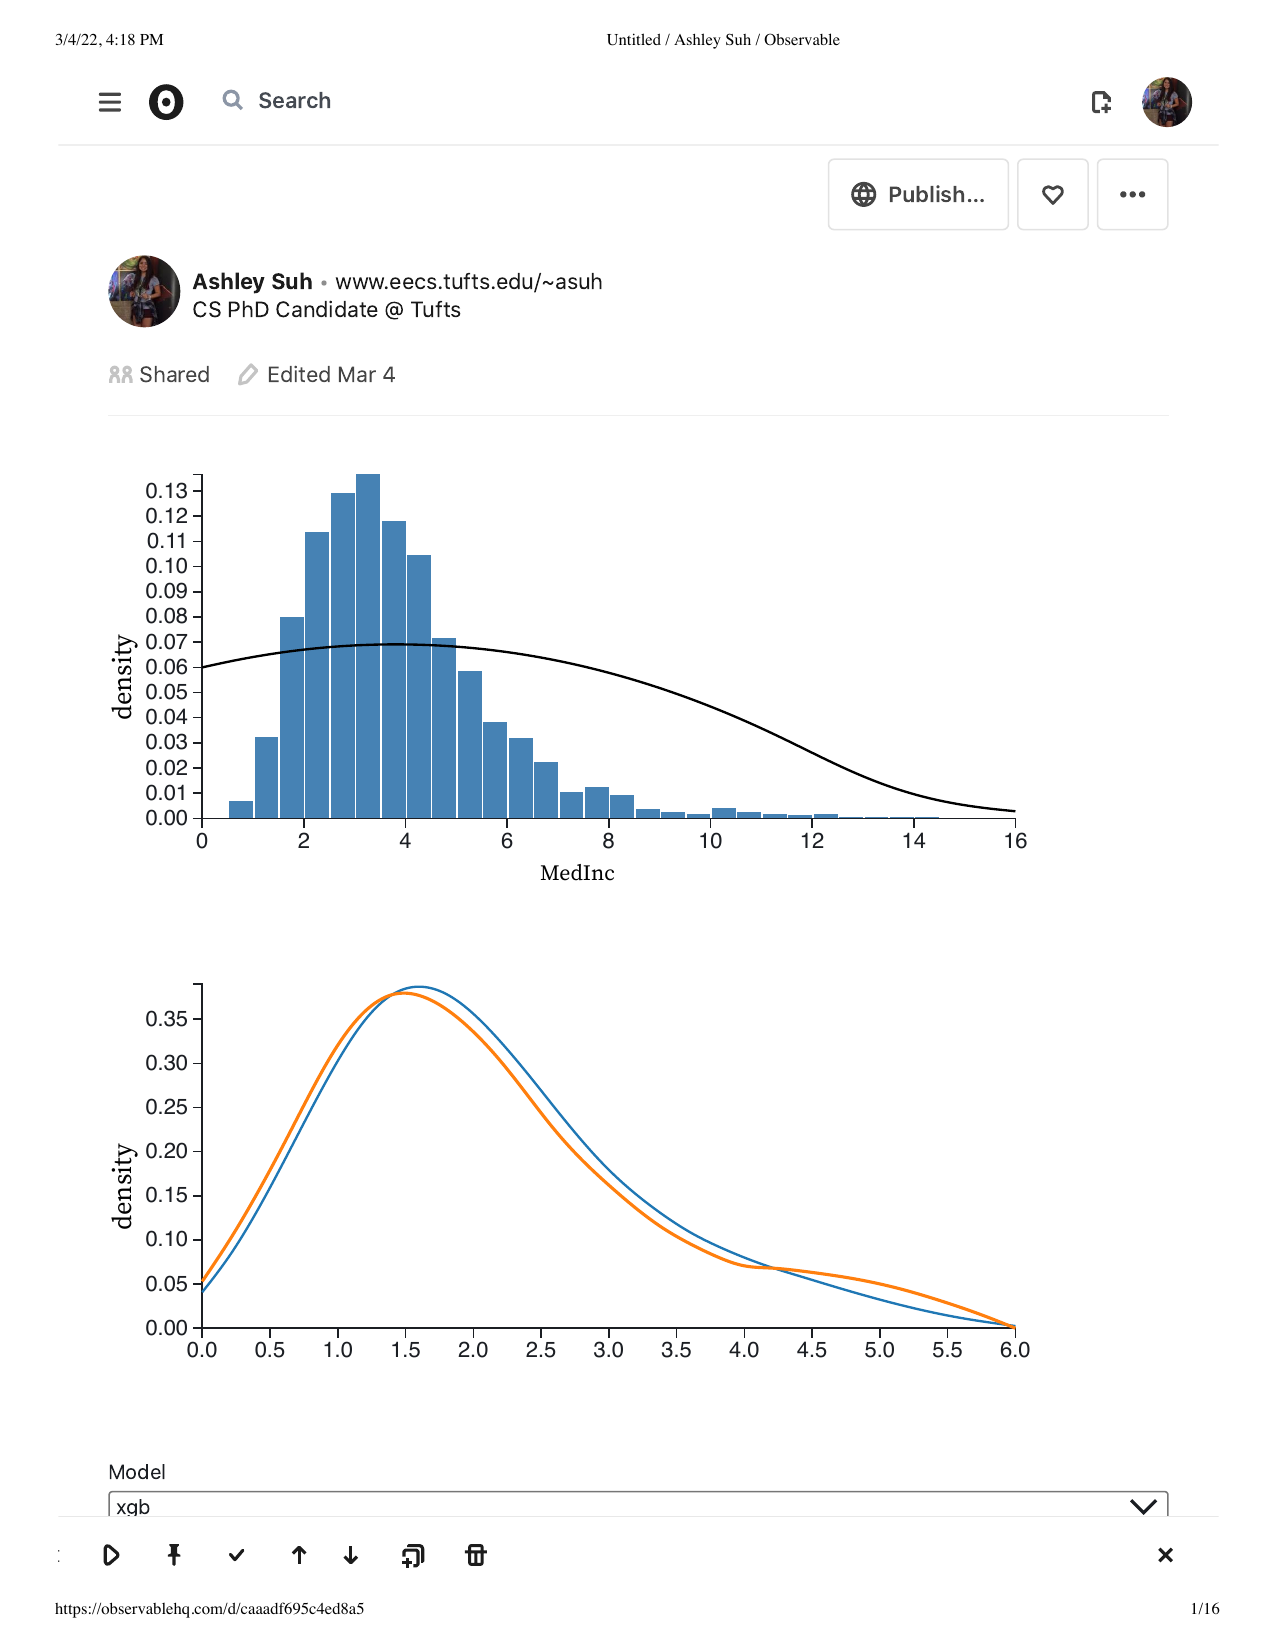} \\ 
    \end{tabular}
    
    \caption{Visualizations to convey overall performance of both models, KNN and XGB. \ashley{Should KNN and XGB have different visual encoding colors for comparison?}}
    \label{fig:global_model_visualizations}
\end{figure*}

% \begin{figure*}[!t]
%     \centering
%     \begin{tabular}{cc}
%     	\toprule

%         \textbf{KNN (Baseline)} & \textbf{XGB (In-development)} \\
        
%         \midrule
        
%     	%%% 1D distribution of predictions
%     	% KNN
%     	\includegraphics[width=.4\linewidth]{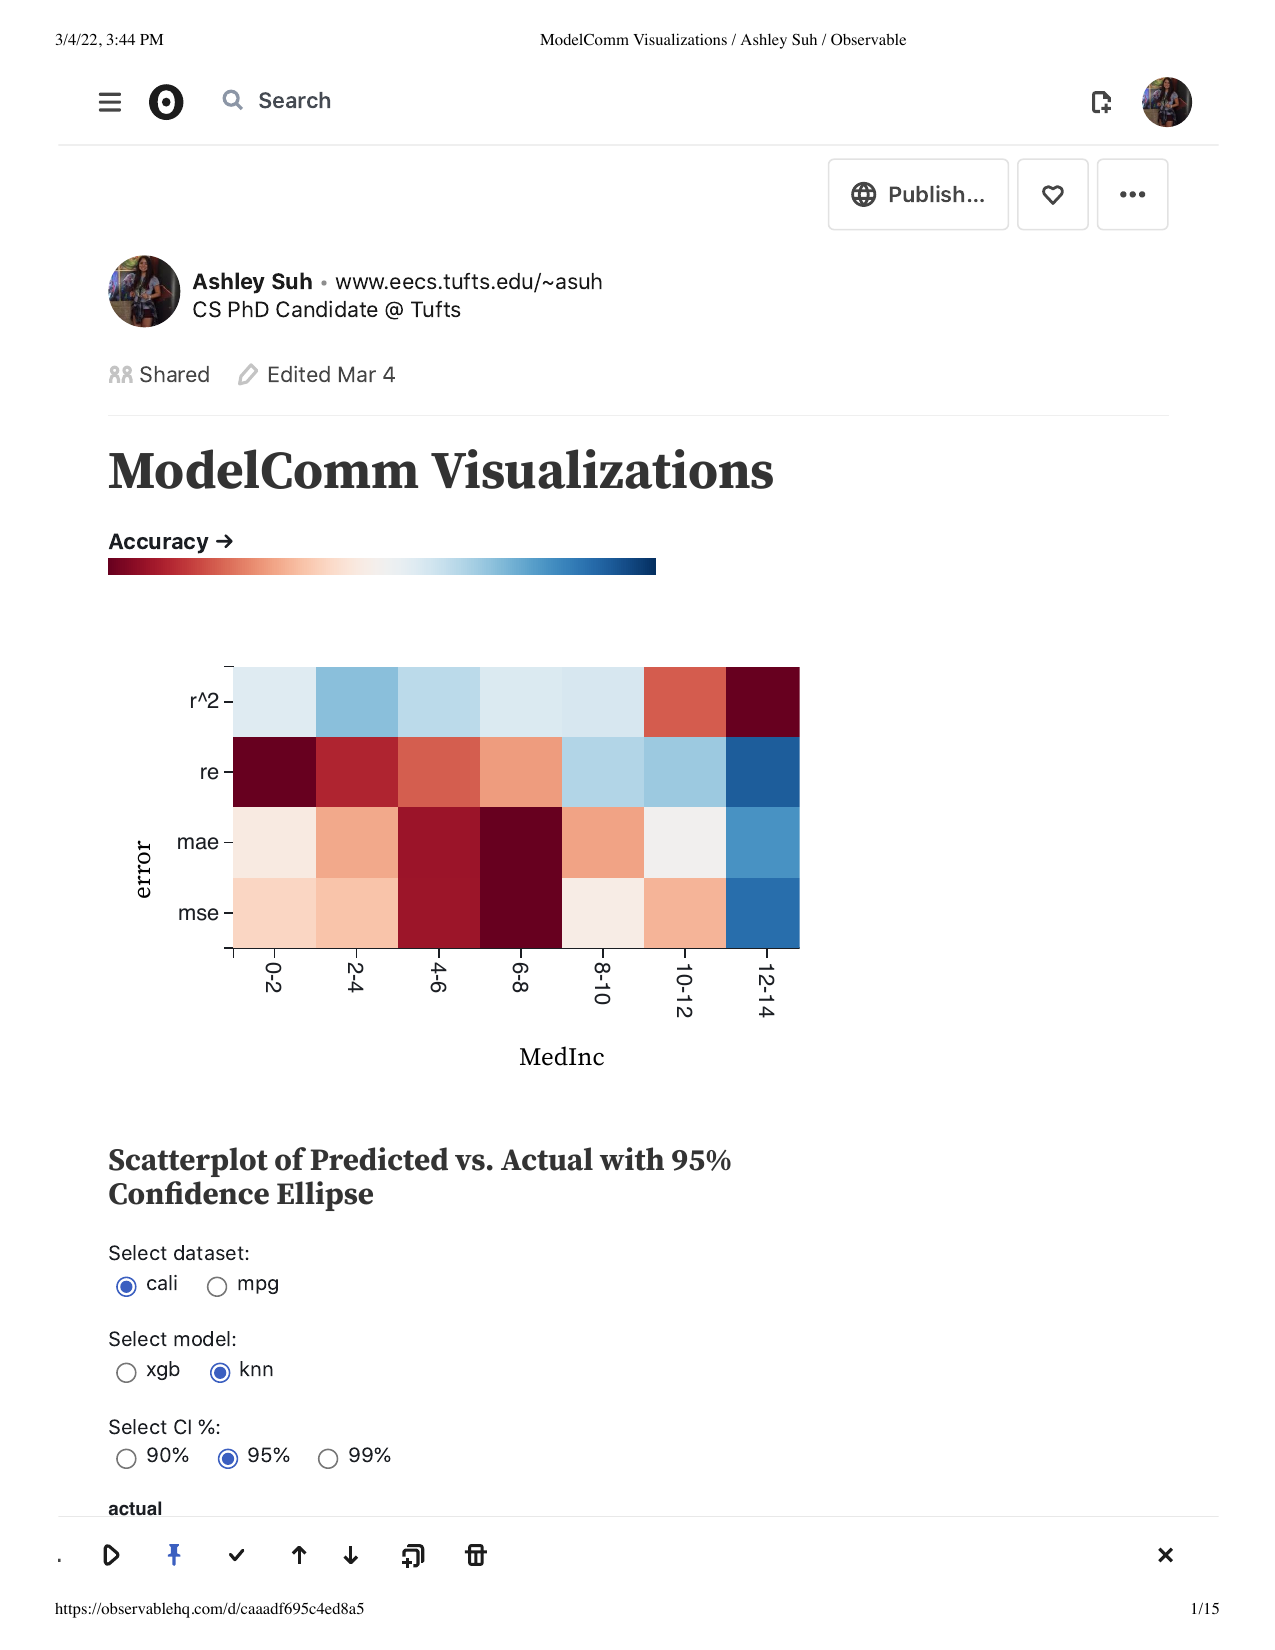}
%     	% XGB
%     	& \includegraphics[width=.4\linewidth]{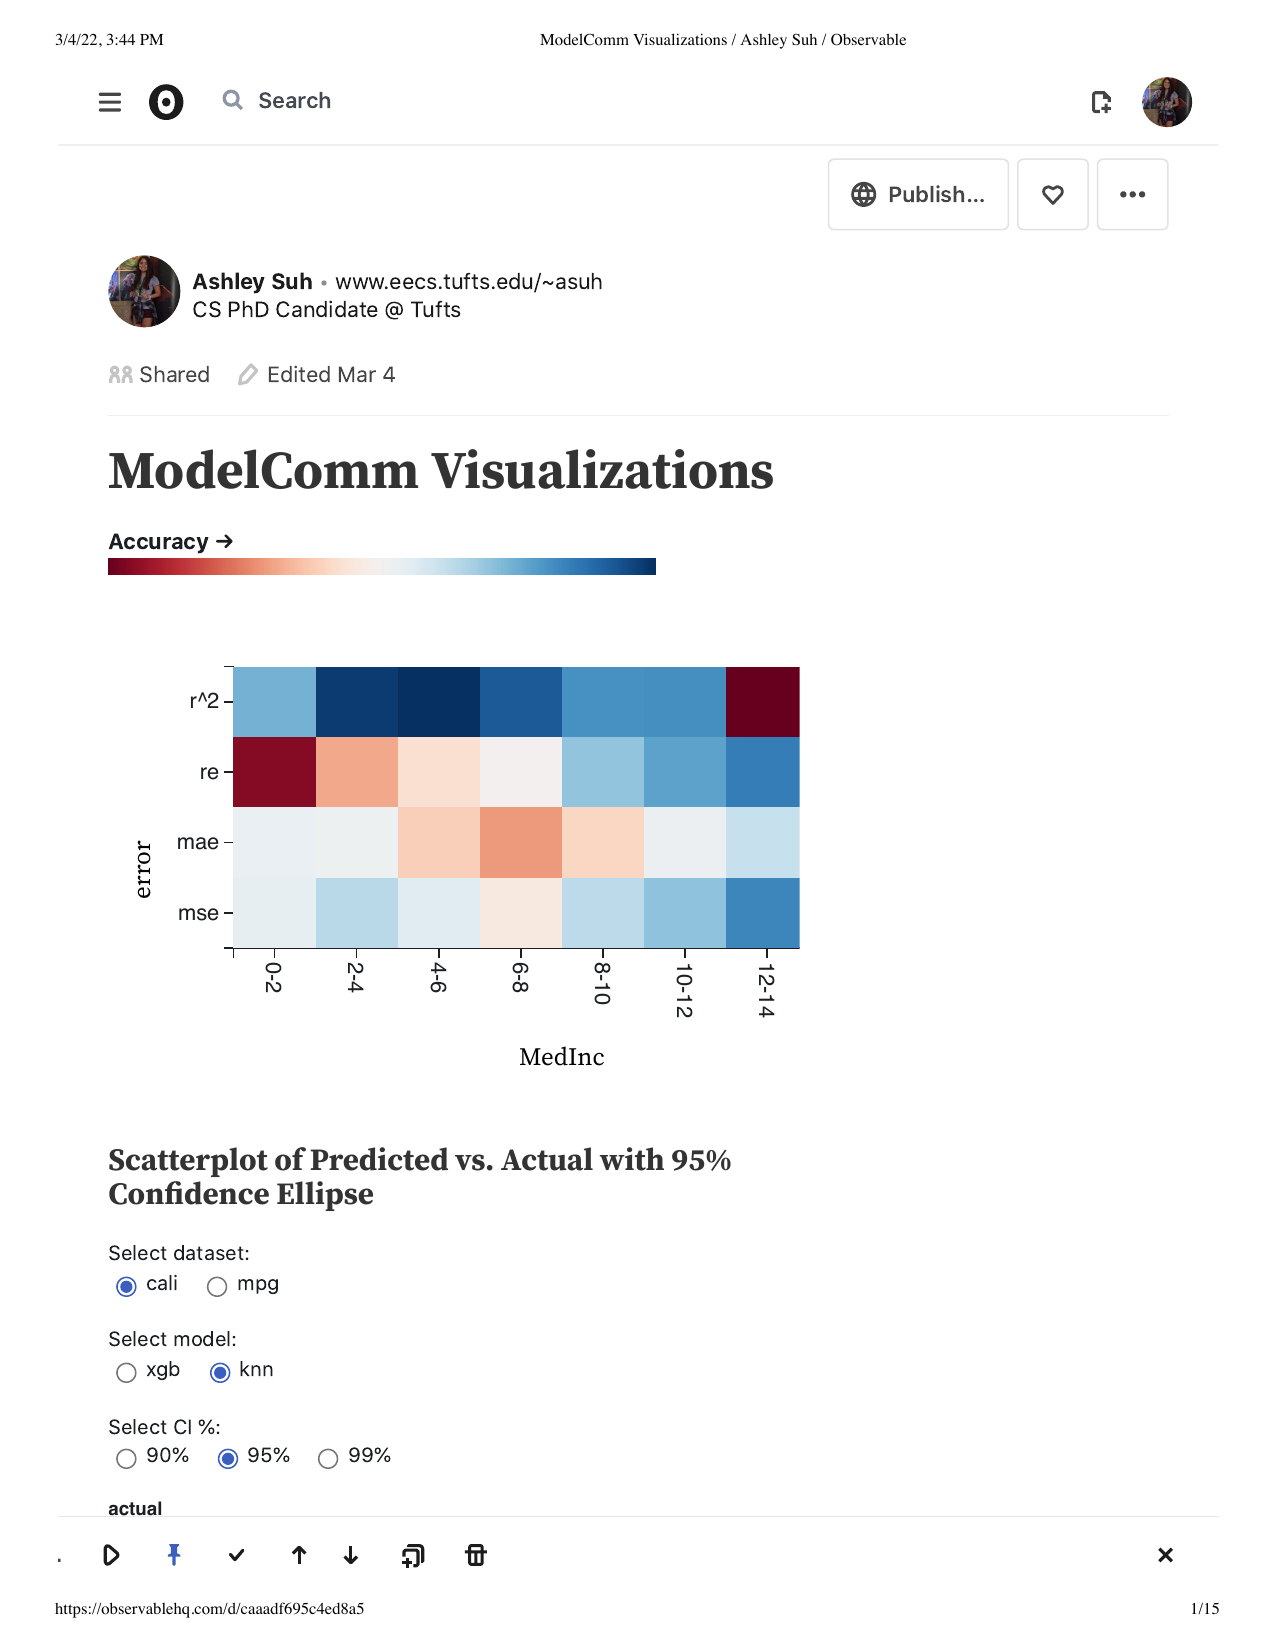} \\ 
    	
%         %%% Corr scatterplot
%     	% KNN
%     	\includegraphics[width=.4\linewidth]{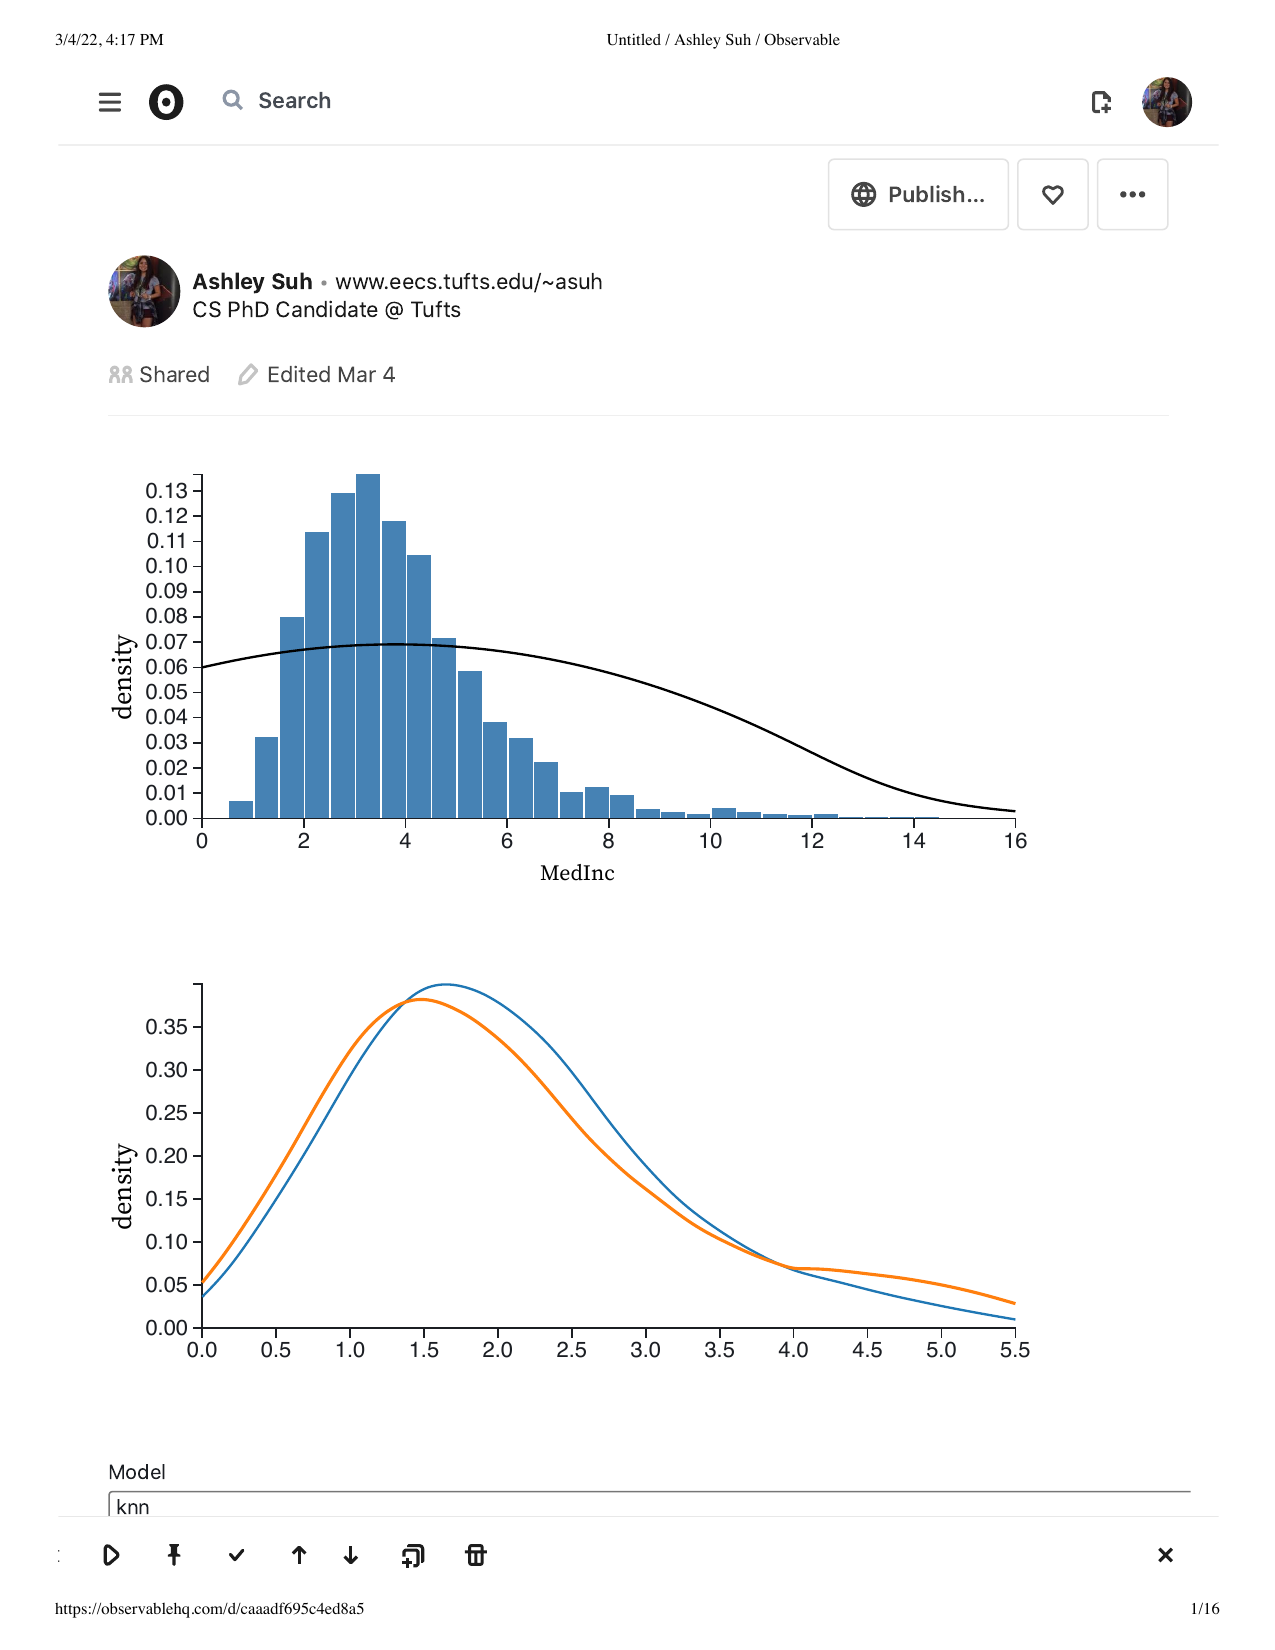}
%     	% XGB
%     	& \includegraphics[width=.4\linewidth]{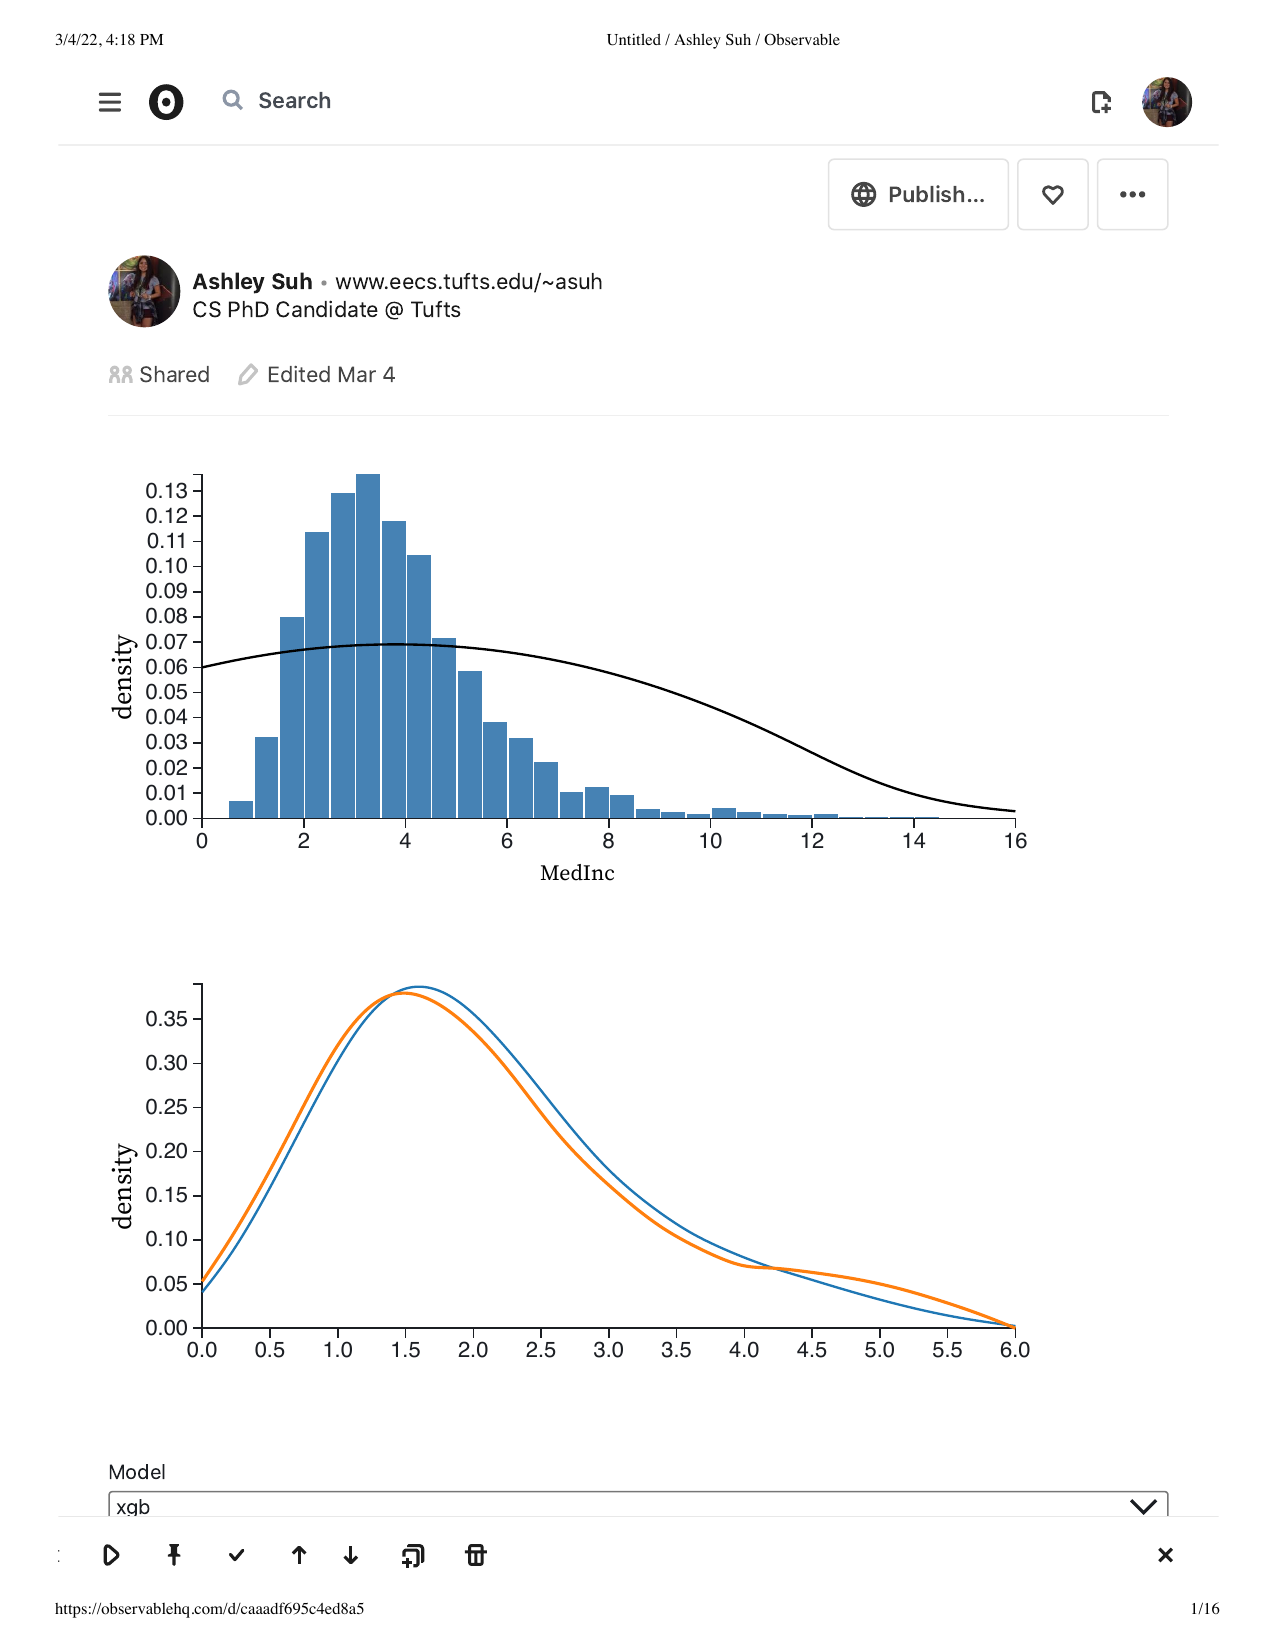} \\ 
    	
%     	%%% Global error bar chart
%     	% KNN
%     	\includegraphics[width=.4\linewidth]{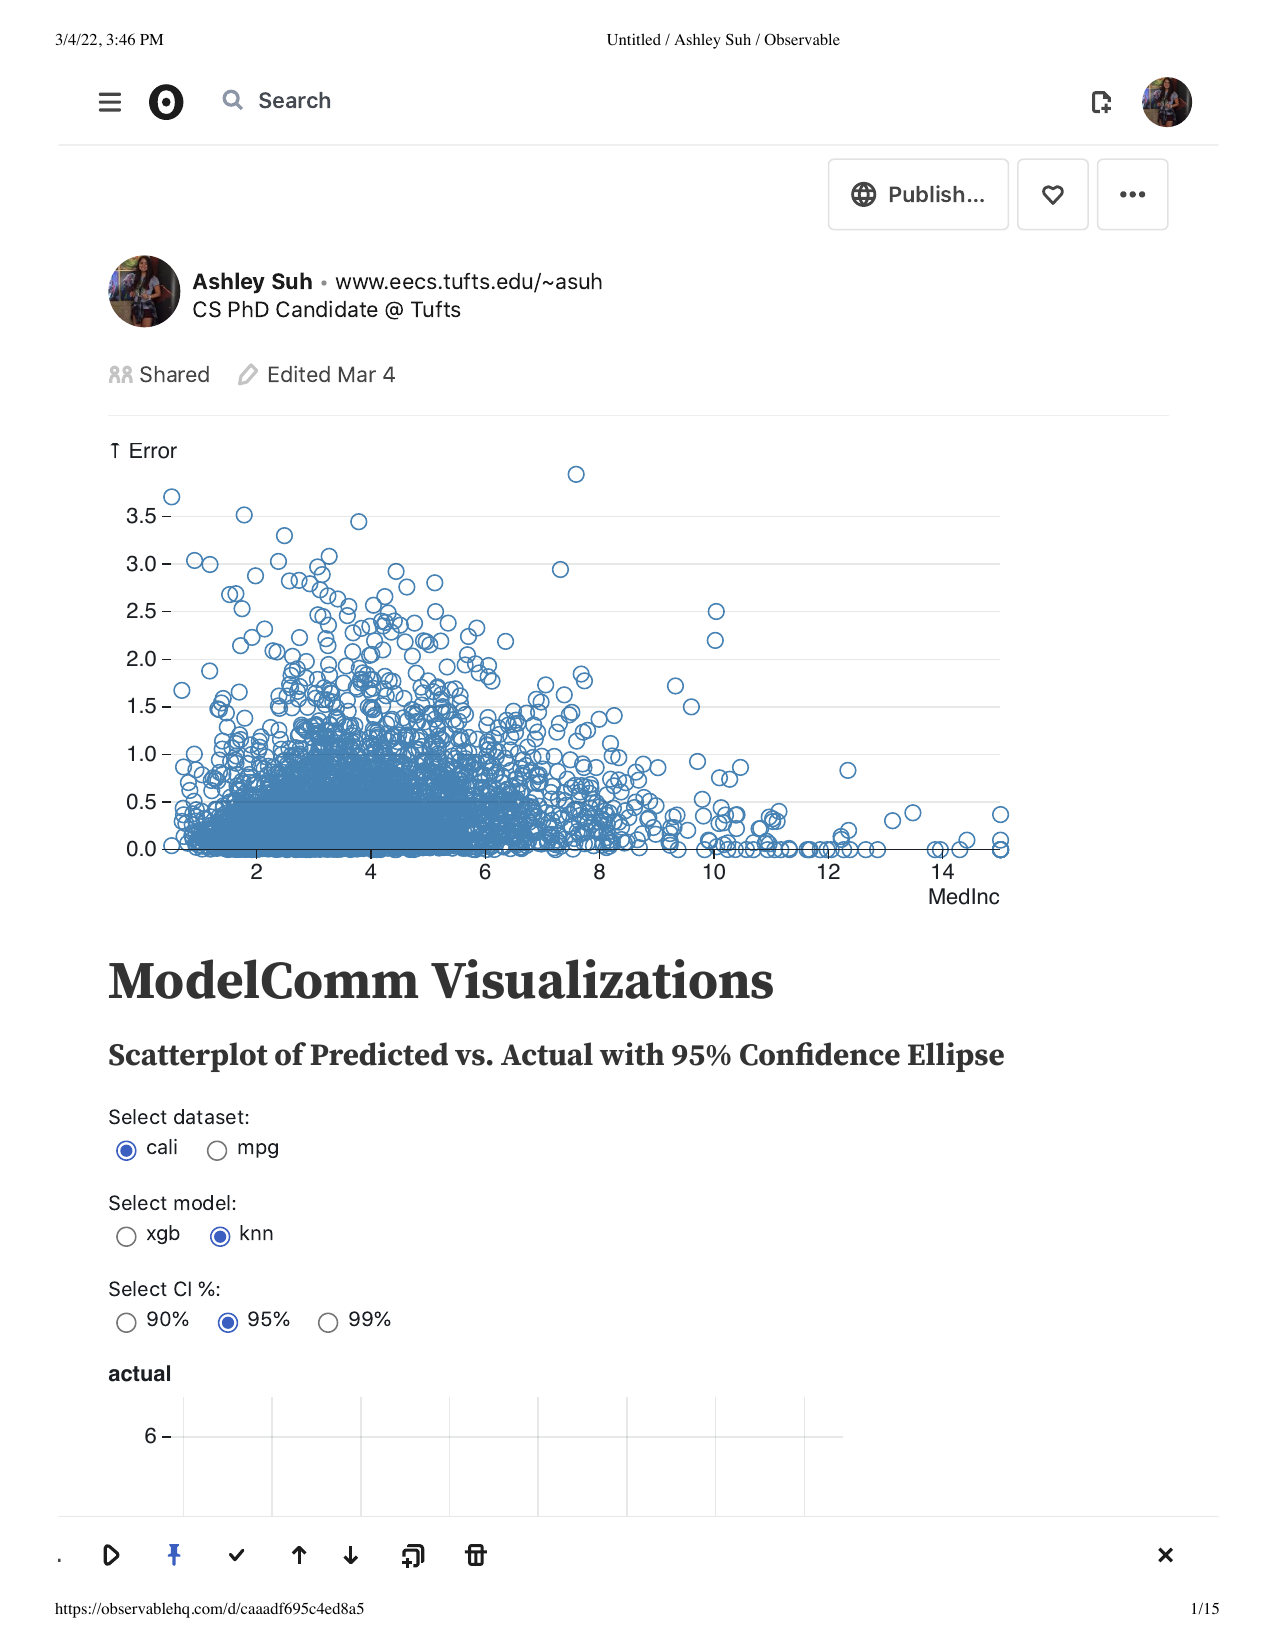}
%     	% XGB
%     	& \includegraphics[width=.4\linewidth]{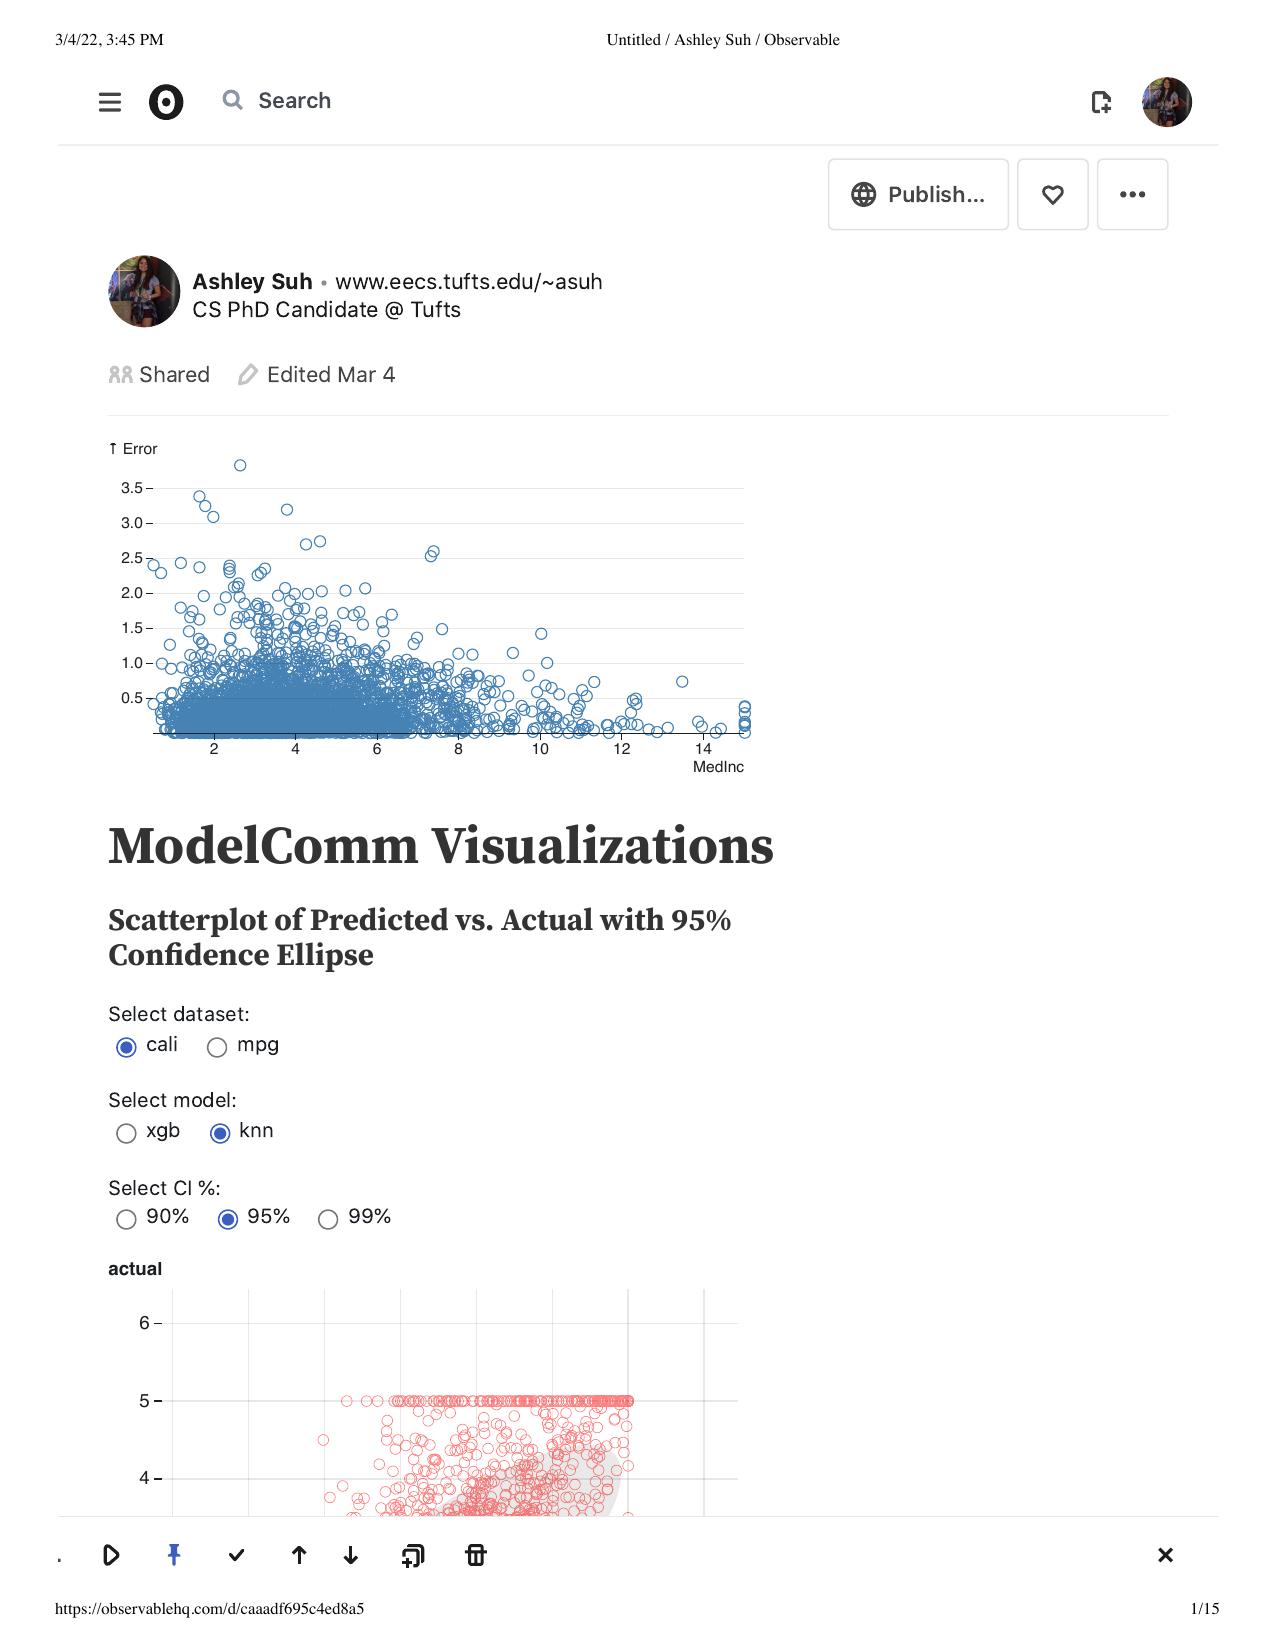} \\ 
    	
%     	%%% Global error bar chart
%     	% KNN
%     	\includegraphics[width=.4\linewidth]{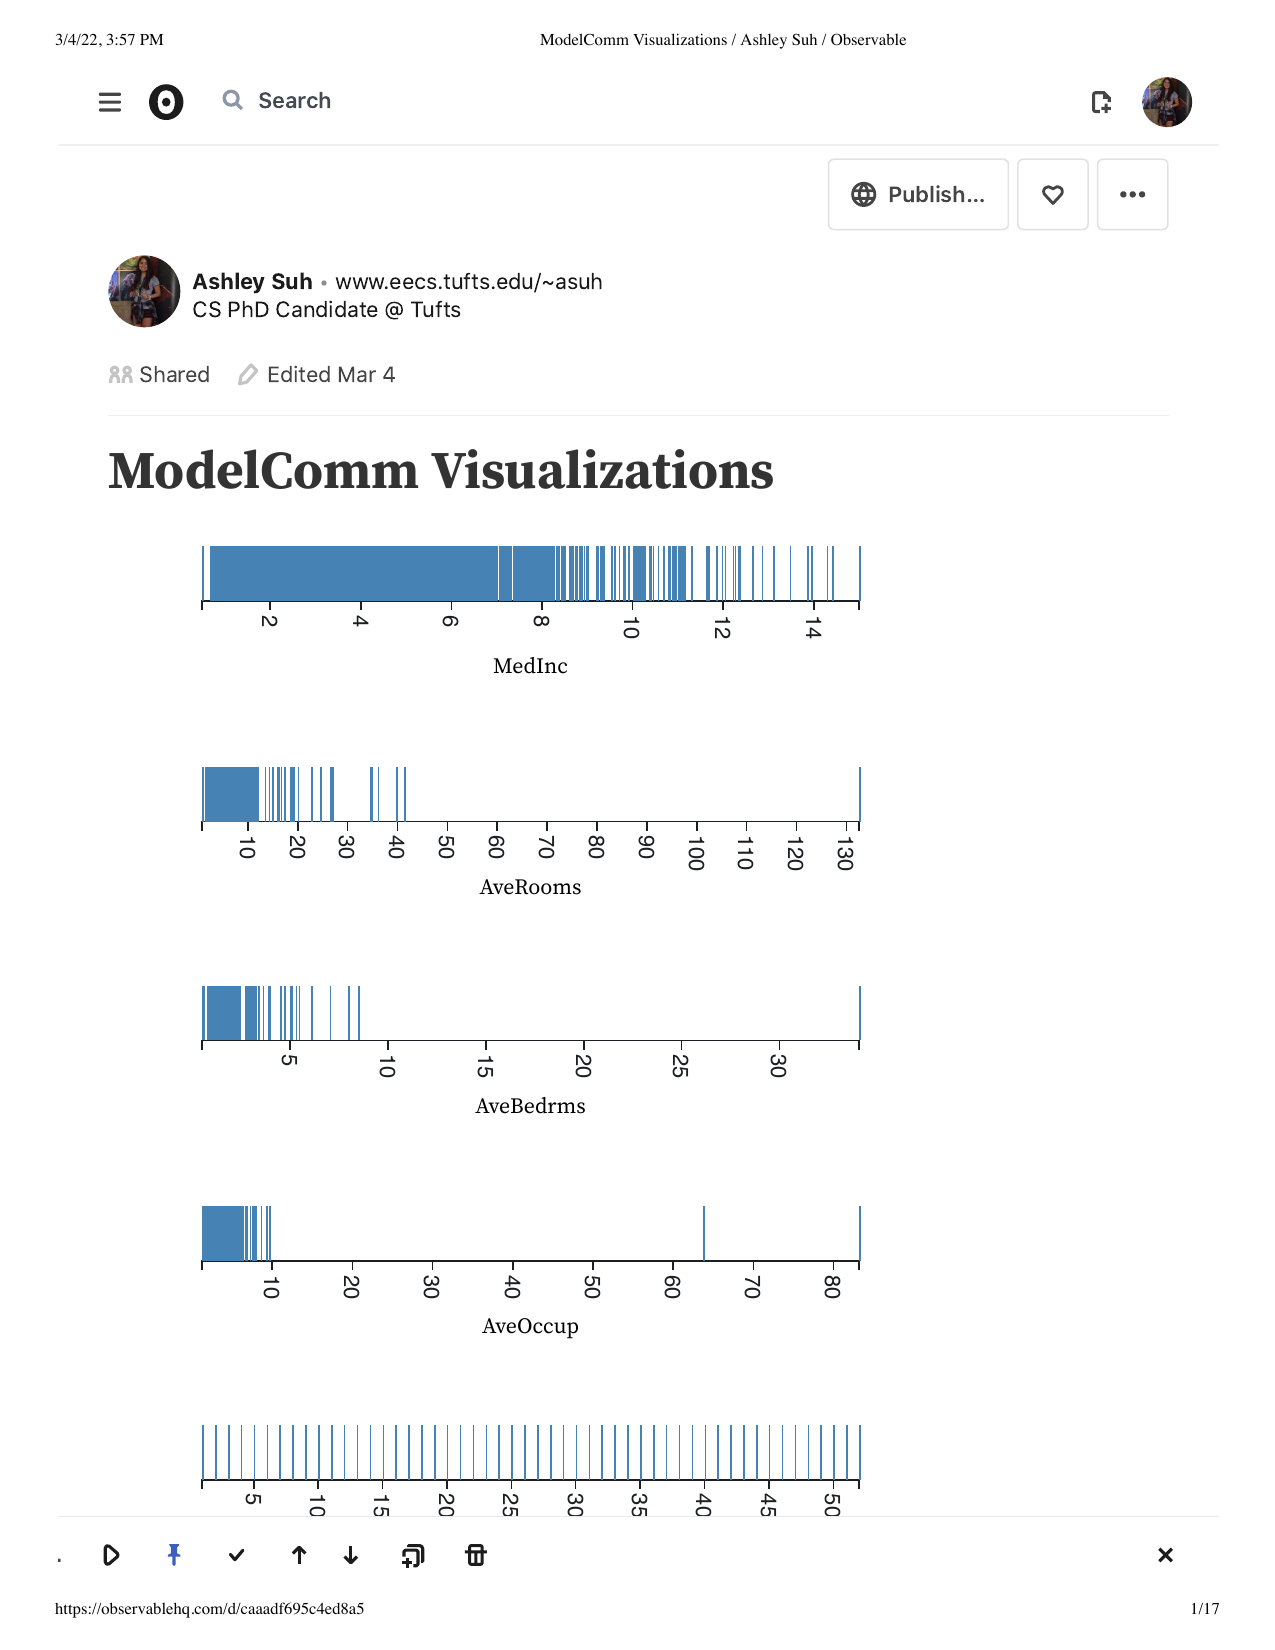}
%     	% XGB
%     	& \includegraphics[width=.4\linewidth]{figures/teaser/cali_barcodes.pdf} \\ 
%     \end{tabular}
    
%     \caption{Visualizations to convey predictive performance of individual features across both KNN and XGB models. We note that some visualizations depict only the distribution of the feature in order to explain potential outliers or anomalies in model performance.}
%     \label{fig:feature_model_visualizations}
% \end{figure*}
